# Supplementary material for: Dissecting Multimodality in VideoQA Transformer Models by Impairing Modality Fusion
Source: arXiv:2306.08889 source file (2024-06-07)
Supplement: Supplementary file 1 [file progressive_quag.tex]

\reba{We apply QUAG progressively to the first $n$ fusion layers of FrozenBiLM to find their relative importance in multimodality. We apply it in the step size of 4 (24 fusion blocks in total) and report the results for ActivityNet-QA (Figure \ref{fig:aqa_prog_quag}) and MSRVTT-QA (Figure \ref{fig:nqa_prog_quag}) Datasets. We consistently find that the first 8 layers are the most important in unimodal interaction and text interactions (and cross-modal interactions as well for ActivityNet-QA).}

\begin{figure}
  \centering
  \includegraphics[width=250]{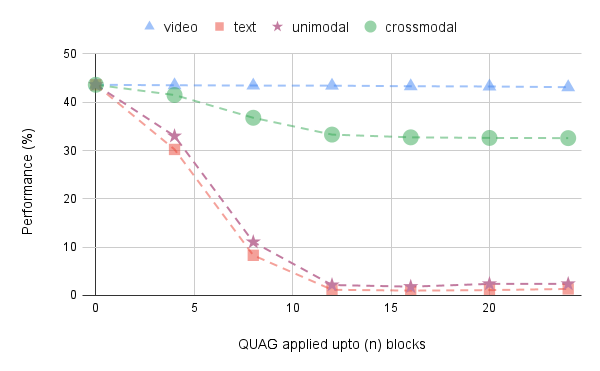}
  \caption{Result of progressive application of QUAG on FrozenBiLM model on ActivityNet-QA dataset}
  \label{fig:aqa_prog_quag}
\end{figure}

\begin{figure}
  \centering
  \includegraphics[width=250]{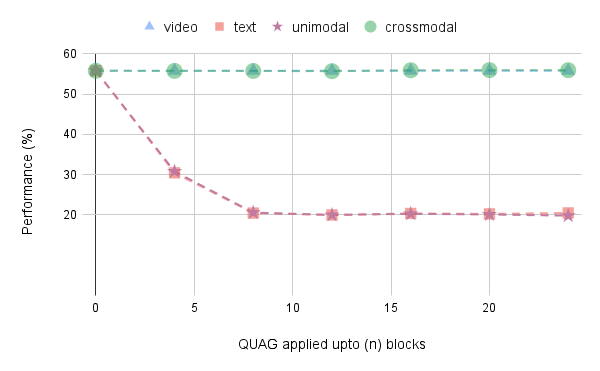}
  \caption{Result of progressive application of QUAG on FrozenBiLM model on NeXT-QA dataset}
  \label{fig:nqa_prog_quag}
\end{figure}
