# Supplementary material for: Dissecting Multimodality in VideoQA Transformer Models by Impairing Modality Fusion
Source: arXiv:2306.08889 source file (2024-06-07)
Supplement: Supplementary file 2 [file supplementary.tex]

% \tableofcontents
\section{QUAG}
% \subsection{Toy Example}
% \input{supp_material/quag_example}
\subsection{Attention Map Visualization}
\input{supp_material/quag_sc_visualization}
\subsection{Code}
\input{supp_material/quag_pseudo_code}
\subsection{Experiment Details}
\input{supp_material/quag_exp}
\subsection{Finegrained Accuracies}
\input{supp_material/quag_fine_acc}
\subsection{Additional Results}
\input{supp_material/additional_quag}
\section{CLAVI}
\subsection{Dataset Creation}
\input{supp_material/clavi_creation}

\subsection{Comparison with Existing Datasets}
\input{supp_material/clavi_comparison}
\subsection{Comprehensive List of Questions}
\input{supp_material/clavi_example}
\subsection{Dataset Metrics}
\input{supp_material/clavi_metrics}
\subsection{Experiment Details}
\input{supp_material/clavi_exp}
\subsection{Fine-grained Accuracies}
\input{supp_material/clavi_fine_acc}
\subsection{Representation Sensitivity Analysis}
\input{supp_material/clavi_additional_analysis}
\subsection{Datasheet} 
\input{supp_material/datasheet}
\newpage
